# Supplementary material for: Electrically Switchable Circular Photogalvanic Effect in Methylammonium Lead Iodide Microcrystals
Source: arXiv:2403.15611 source file (2024-03-22)
Supplement: Supplementary file 1 [file Perovskite_CPGE_SM.pdf]

# Supplementary Information for Electrically Switchable Circular Photogalvanic Effect in Methylammonium Lead Iodide Microcrystals

Yuqing Zhu[1], Ziyi Song[1], Rodrigo Becerra Silva[1], Bob Minyu Wang[1], Henry Clark Travaglini[1], Andrew C Grieder[2], Yuan Ping[2], Liang Z. Tan[3], and Dong Yu[1]

[1]Department of Physics and Astronomy, University of California, Davis
[2]Department of Materials Science and Engineering, University of Wisconsin-Madison
[3]Molecular Foundry, Lawrence Berkeley National Lab

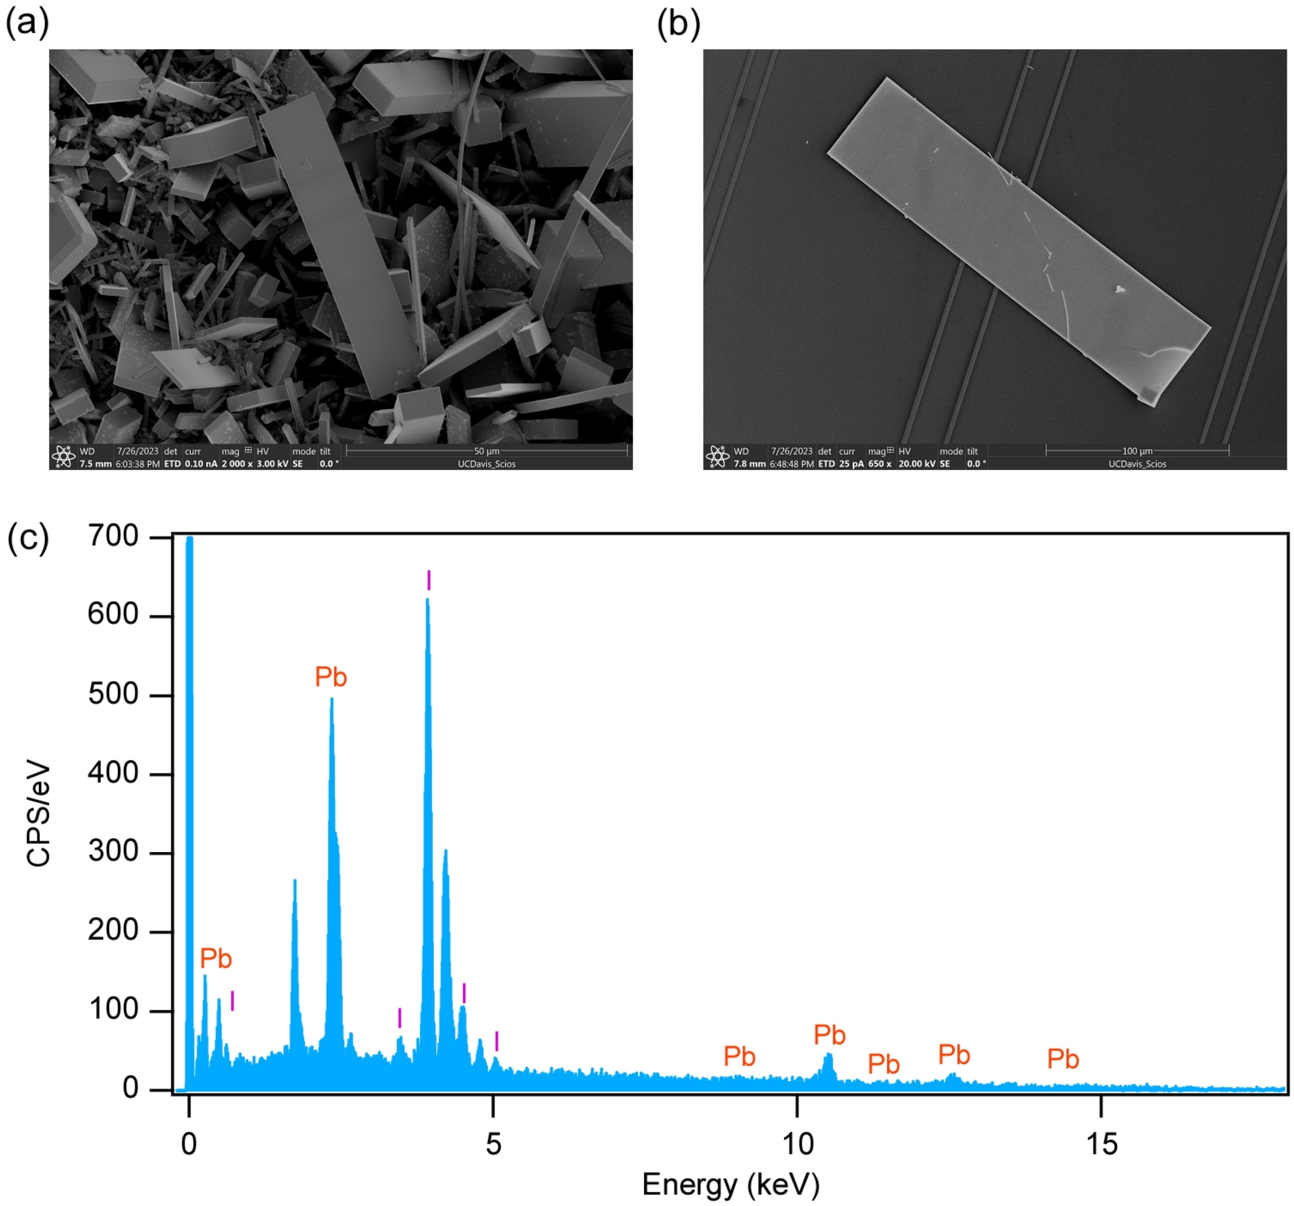


**Figure S 1.** $MAPbI_3$ microcrystal growth and characterization. Scanning electron micrograph of (a) the growth substrate and (b) the transferred crystal on a pair of gold electrodes. (c) EDS result of the device; the Pb to I atomic ratio is 26% to 74%, which agrees well with the expected value of 1 to 3.

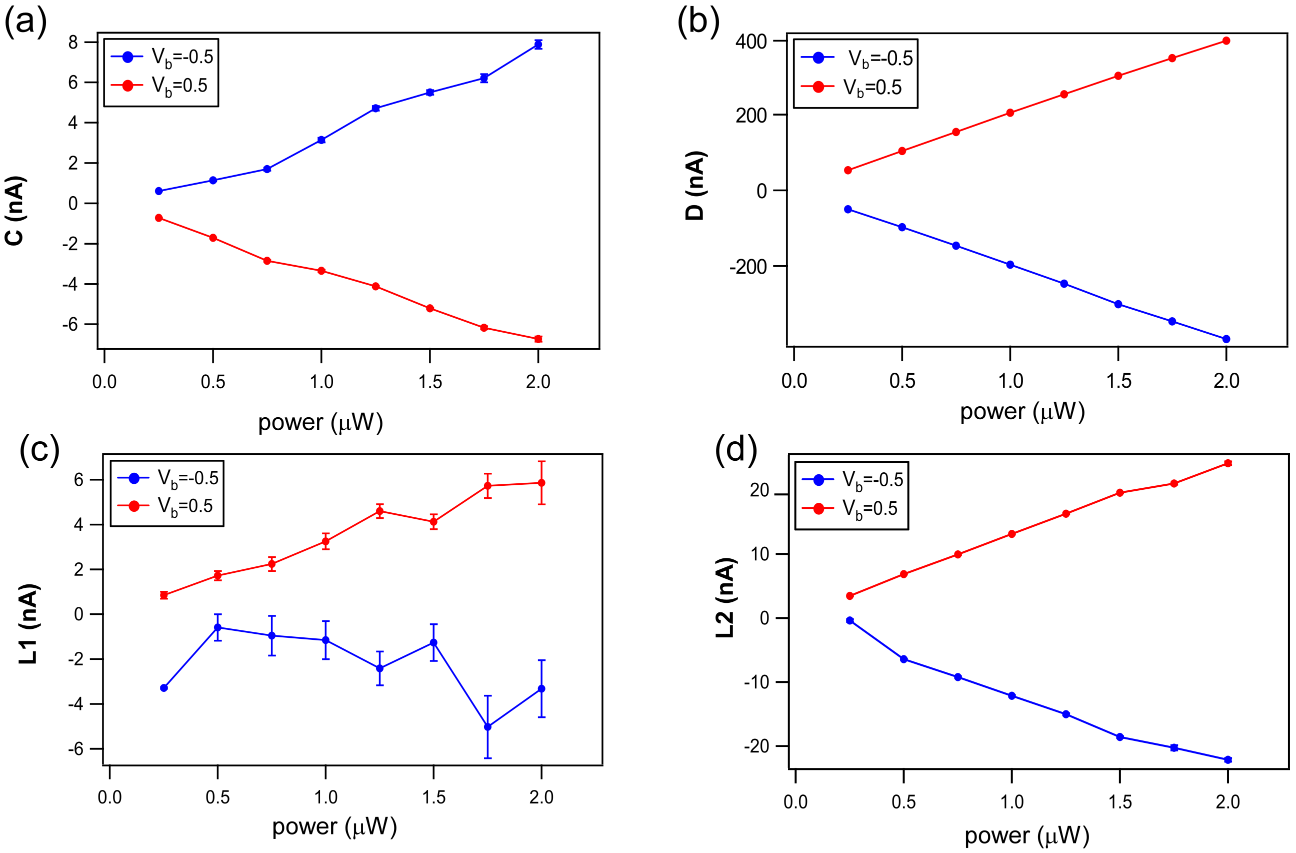


**Figure S 2.** Fitting parameters of photocurrent as functions of laser power at 80K. Extracted (a) C, (b) D, (c) L1, and (d) L2 values are largely linear with the laser power.

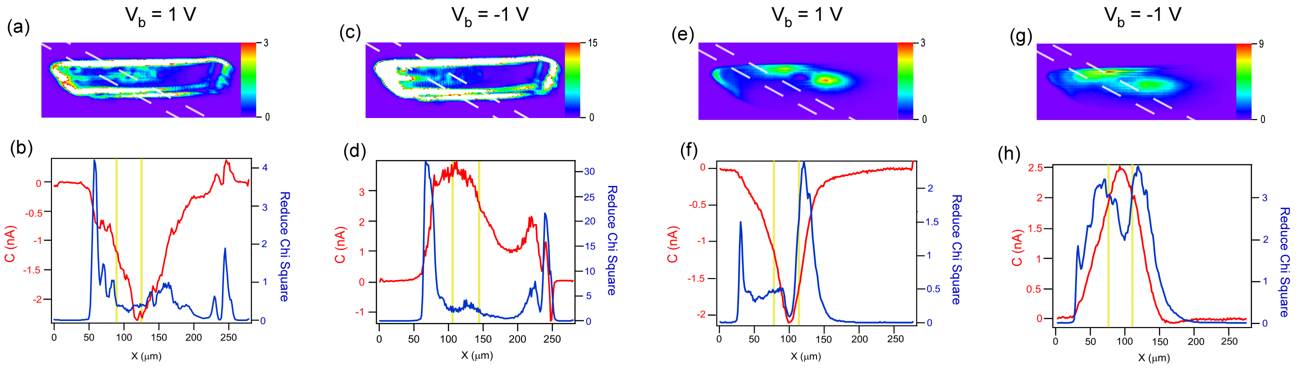


**Figure S 3.** Maps and cross-section of the reduced chi-square from the fitting of Fig. 2 in the main text. Error analysis shows that the extracted fitting parameters are unreliable on the crystal edge. The large extracted $C$ values on the crystal edge are likely due to the rapid photocurrent change when the laser moves on and off the crystal and hence are not reliable. However, the reduced chi-square is reasonable away from the edge. (a)-(d) are at 78 K and (e)-(h) are at 270 K.

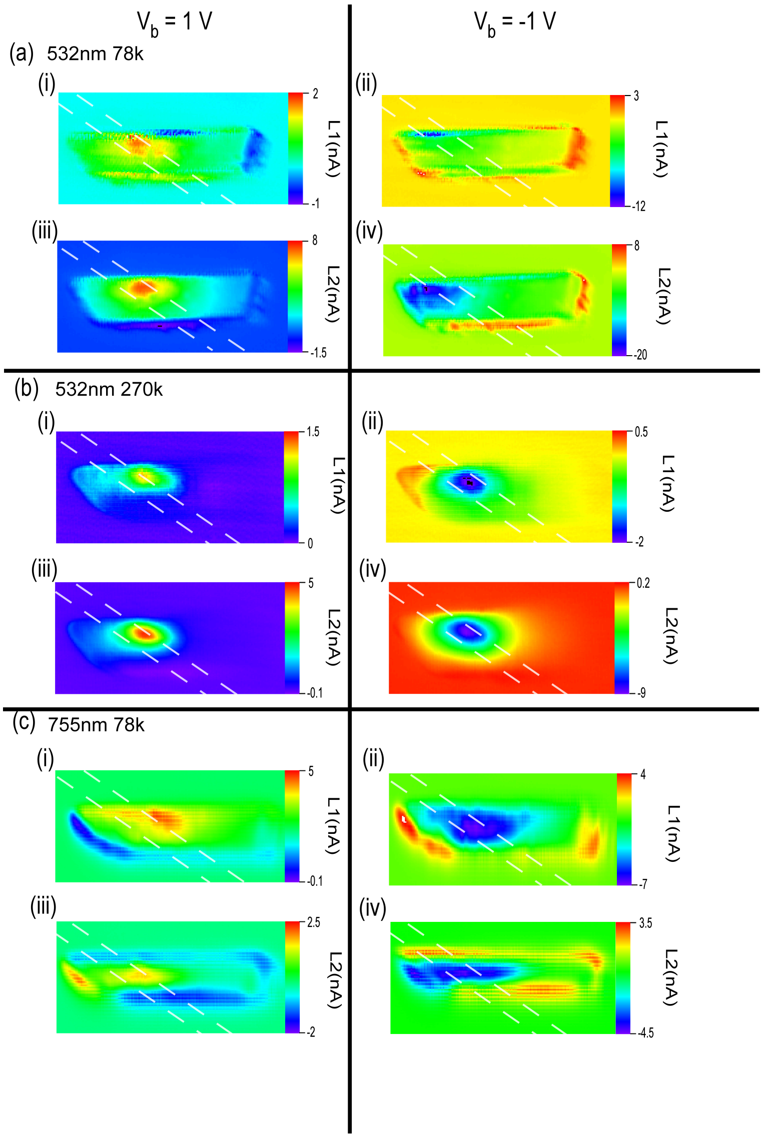


**Figure S 4.** Extracted L1, L2 maps at $V_b = \pm 1$ V with (a) laser wavelength of 532 nm at 78 K, (b) 532 nm at 270 K, and (c) 755 nm at 78 K.

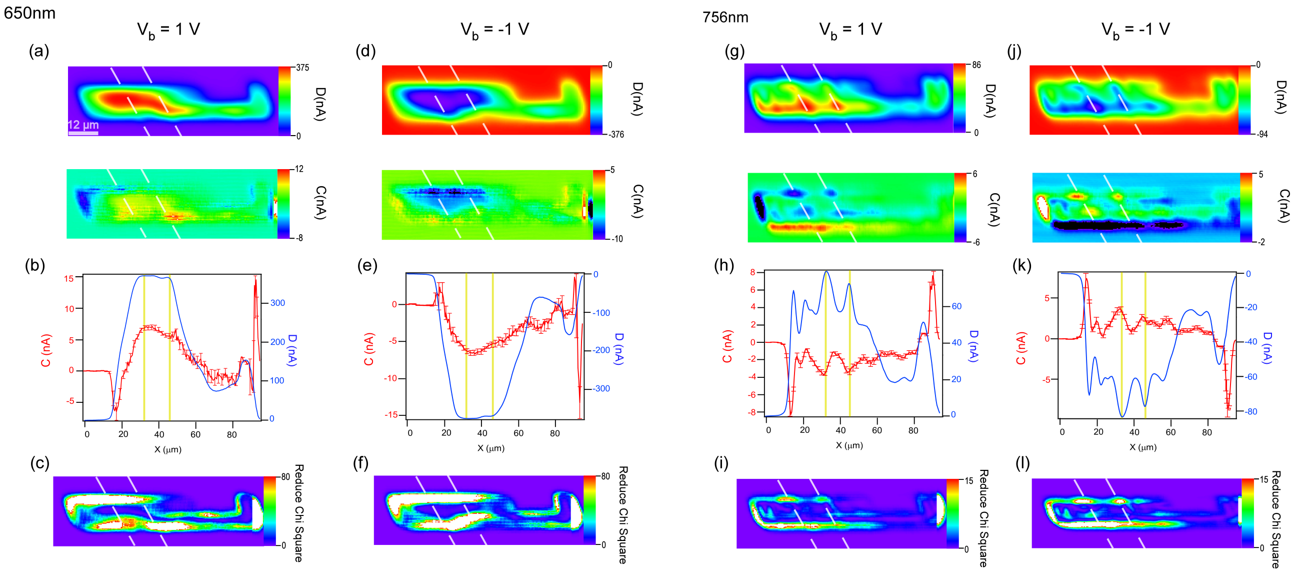


**Figure S 5.** Spatially resolved CPGE at 78K with $V_b = \pm$ 1 V on a second device. The shape of the crystal is not regular but the CPGE result is consistent with the first device.

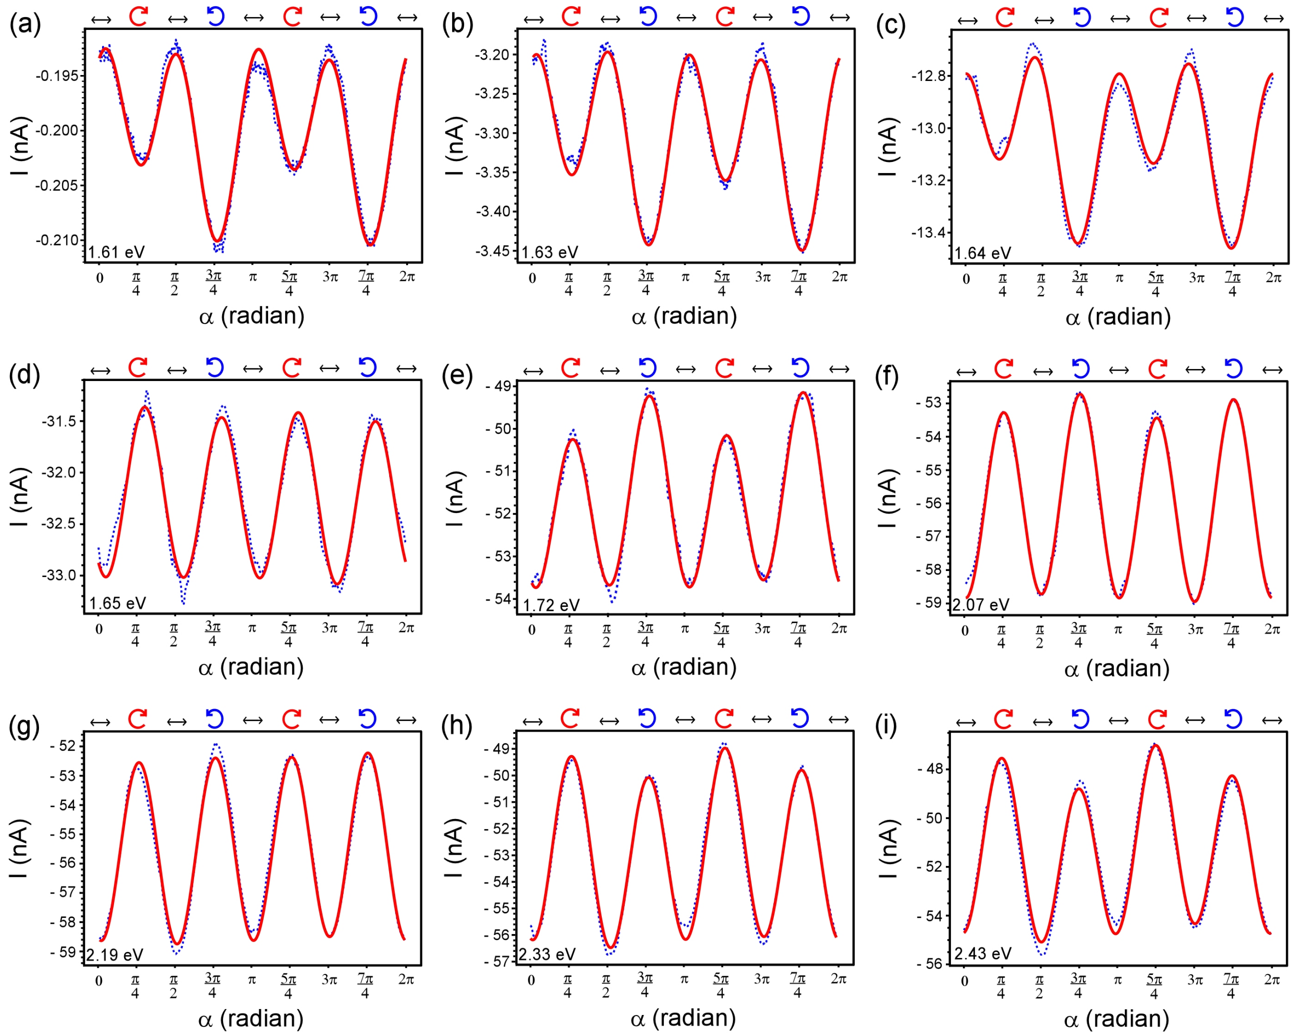


**Figure S 6.** Photocurrent as a function of the QWP angle $\alpha$ at various photon energy from 1.61 eV to 2.43 eV at 80K. Notice that $C$ is positive below 1.65 eV (bandgap), then stays negative in the range of 1.65 eV and 2.19 eV, and finally transitions back to positive above 2.19 eV. The $C$ value extracted from the fitting as a function of the photon energy can be found in Fig. 3(c) in the main text.

755nm, 79K

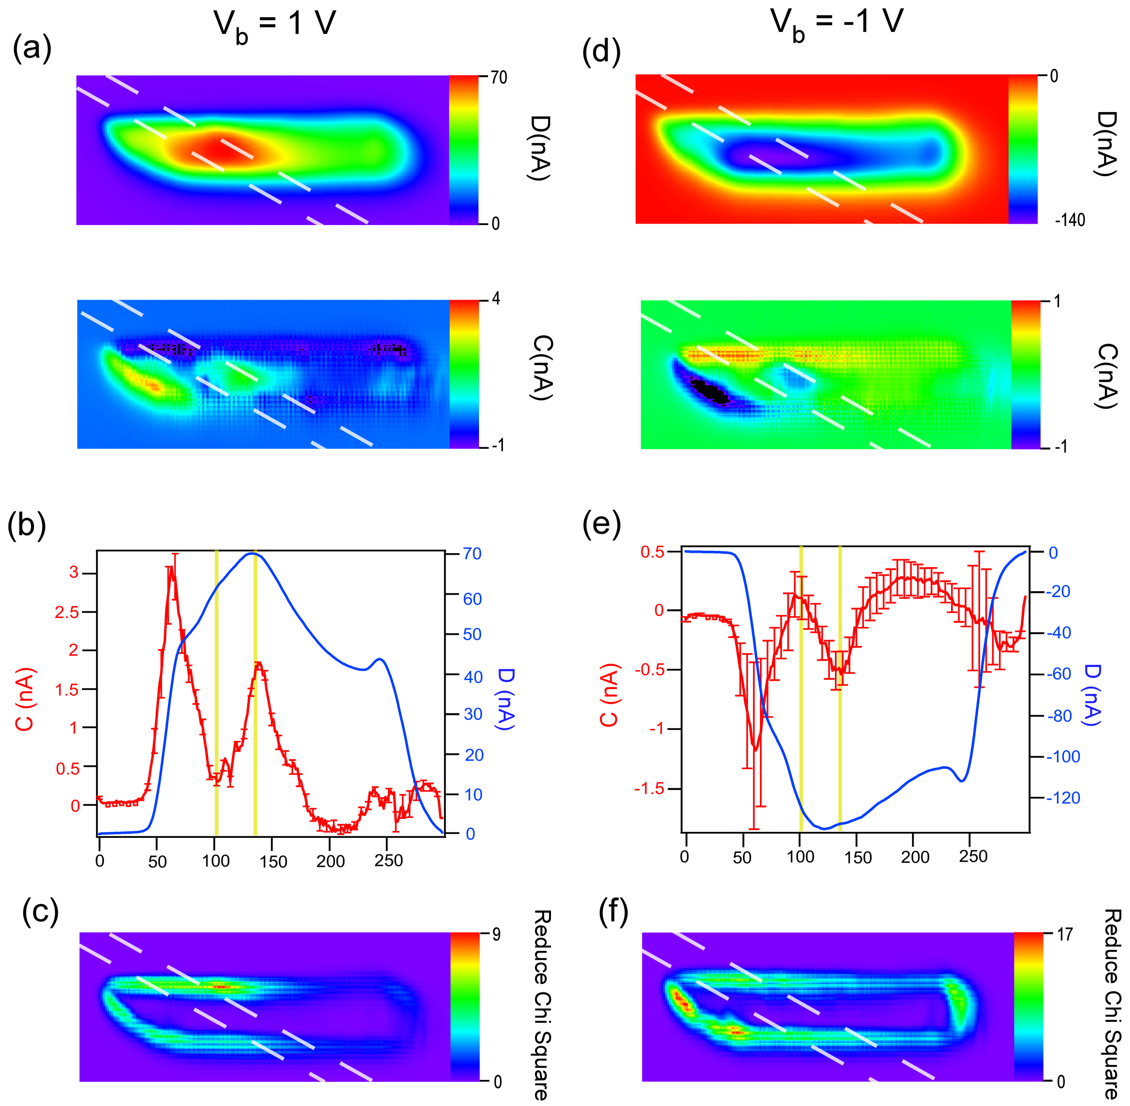


**Figure S 7.** Spatially resolved CPGE at 79k with $V_b = \pm 1$ V and laser wavelength of 755 nm. The sign of $C/D$ is opposite to that with laser wavelength of 532 nm which is consistent with our wavelength-dependent data. (c) and (f) shows that the reduced chi-square value is large on the crystal edge.

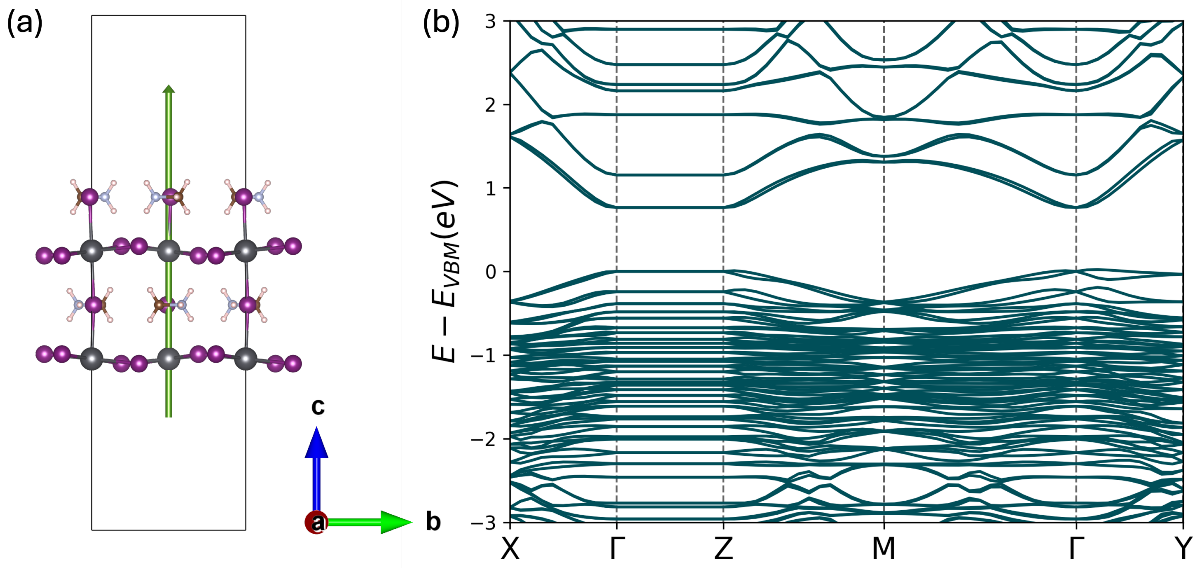


**Figure S 8.** Fully relaxed ionic positions (a) and band structure (b) for the (001) MAPI slab calculated by DFT with spin-orbit coupling. Green arrow indicates the approximate $C_{4v}$ axis for the inorganic ions as discussed in the main text.

# 1 Density Functional Theory (DFT)

Structural and electronic properties were computed using Density Function Theory (DFT). Open Source plane-wave package Quantum ESPRESSO[4] was used for structure optimization with Perdew-Burke-Ernzerhof (PBE) exchange correlation functionals with GBRV pseudopotentials[3]. For all structural optimizations the ionic positions were relaxed until all forces on ions were below 0.001 Ry/Bohr. First the bulk orthorhombic methyl-ammonium lead iodide perovskite (MAPI) structure was optimized. The optimized bulk structure was used to construct the asymmetric slab terminated along the (001) surface with a 10 Å vacuum layer. Finally, the ion positions in the slab were then relaxed and the structure can be seen in Fig. S8(a). Electronic properties were computed using PBE exchange correlation functionals including spin-orbit coupling (SOC) with norm conserving full relativistic pseudopotentials from PseudoDojo[8]. The band structure and dipole matrix elements were computed using software package JDFTx[7] from the optimized slab structure. The ab-initio CPGE tensor and photocurrents were implemented numerically in the in-house code interfaced with JDFTx.

## 1.1 DFT second order injection current

The CPGE tensor, second order injection current density, and current were computed using equation S1, S2, and S3 respectively[6]:

$$\beta_{ij} = \frac{e^3\pi}{N_{\boldsymbol{k}}V\hbar}\epsilon_{jkl}\sum_{\boldsymbol{k},n,m} f^{\boldsymbol{k}}_{nm}\Delta^i_{\boldsymbol{k},nm}r^k_{\boldsymbol{k},nm}r^l_{\boldsymbol{k},mn}\delta(\hbar\omega - E_{\boldsymbol{k},nm}) \tag{S1}$$

$$j_i = \tau\beta_{ij}(E(\omega)\times E^*(\omega))_j \tag{S2}$$

$$C_i = j_iA_{cross} \tag{S3}$$

where $n$ and $m$ are band indices and $i$, $j$, $k$, and $l$ are Cartesian directions. Here $f_{\boldsymbol{k},nm}$ occupation difference, $E_{\boldsymbol{k},nm}$ is the energy difference, $r_{\boldsymbol{k},nm}$ are the dipole-matrix elements, and $\Delta_{\boldsymbol{k},nm}$ are the difference in velocity-matrix elements of band $n$ and $m$ at k-point $\boldsymbol{k}$ respectively. All these elements are computed from DFT directly. Here we use a relaxation time ($\tau$) of 164 fs computed for a previous study in methyl ammonium lead bromide perovskite ($MAPbBr_3$).[9] To calculate the current density, we use the optical electric field ($E$) from experiment and to convert from current density ($j_x$) to current ($C_x$) we use the cross section ($A_{cross}$) of 0.5 $\mu m^2$. As the CPGE occurs at the surface, we estimate the surface layer thickness by using a Debye length on the order of 100 nm. Then the relevant cross section area at the top surface is 5 $\mu$m $\times$ 100 nm. The angle dependence of CPGE is computed in Fig. S9. Here we have enforced the $C_{4v}$ point group symmetry of the CPGE tensor. To match the experimental angle convention, 0° is normal to the surface in our model. To be consistent with experimental incident angle and laser energy, an angle of 45° and a photon wavelength of 650 nm are used, which result in a photocurrent 0.028 nA in our calculations (also reported in main text). To test the effect of slab thickness we also compute the $\beta$ for a thicker slab (4 layer in Fig 10). All of the qualitative trends are consistent for both the thinner and thicker slab.

## 1.2 Rashba band fitting

To inform the 4 band model of the third-order injection current (discussed below) we fit the DFT band structure to the Rashba band splitting model:

$$E(k) = E_0 + \frac{\hbar^2k^2}{2m^*} \pm \alpha k, \tag{S4}$$

where $E_0$ is the energy offset, $m^*$ is the band mass, and $\alpha$ is the Rashba splitting parameter. The fitting results are plotted in Fig. S11. The conduction and valence bands were fit in both the $k_x$ and $k_y$

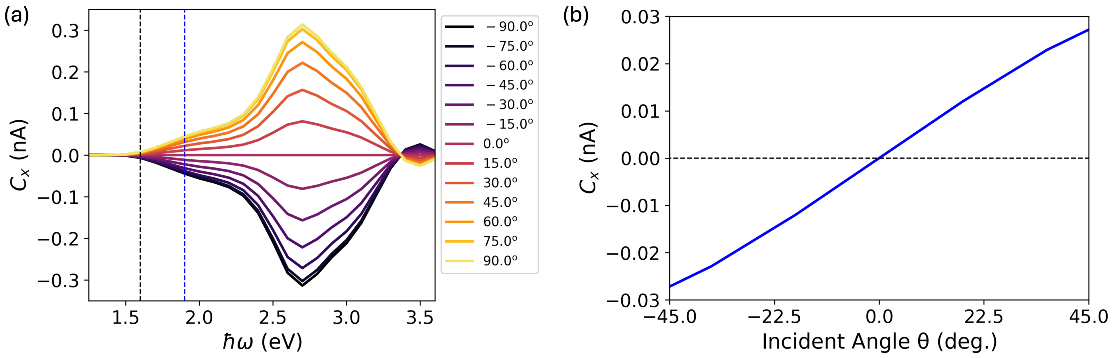


**Figure S 9.** Angle and frequency dependence of the CPGE photocurrent. The angle is between the light propagating and the current collection directions. Current collection is fixed in the x direction while light propagation is varied in the yz plane with zero degree as the z direction. (a) The photocurrent as a function of photon energy (with the band-gap marked by the dashed black line). To account for the underestimation of the DFT band gap we shift the CPGE spectra by the difference between the experimental (1.66 eV) and DFT (0.76 eV) band-gaps. (b) The angle dependence of photocurrent at a wavelength of 650 nm, indicated in (a) by a dashed blue line. We can find at an angle of 45° and a photon wavelength of 650 nm, a photocurrent of 0.028 nA is obtained in our calculation.

directions. All the points were used in the fits except for the valence bands in the $k_y$ direction, where we use the range of DFT data which minimized the error in the least square's fit.

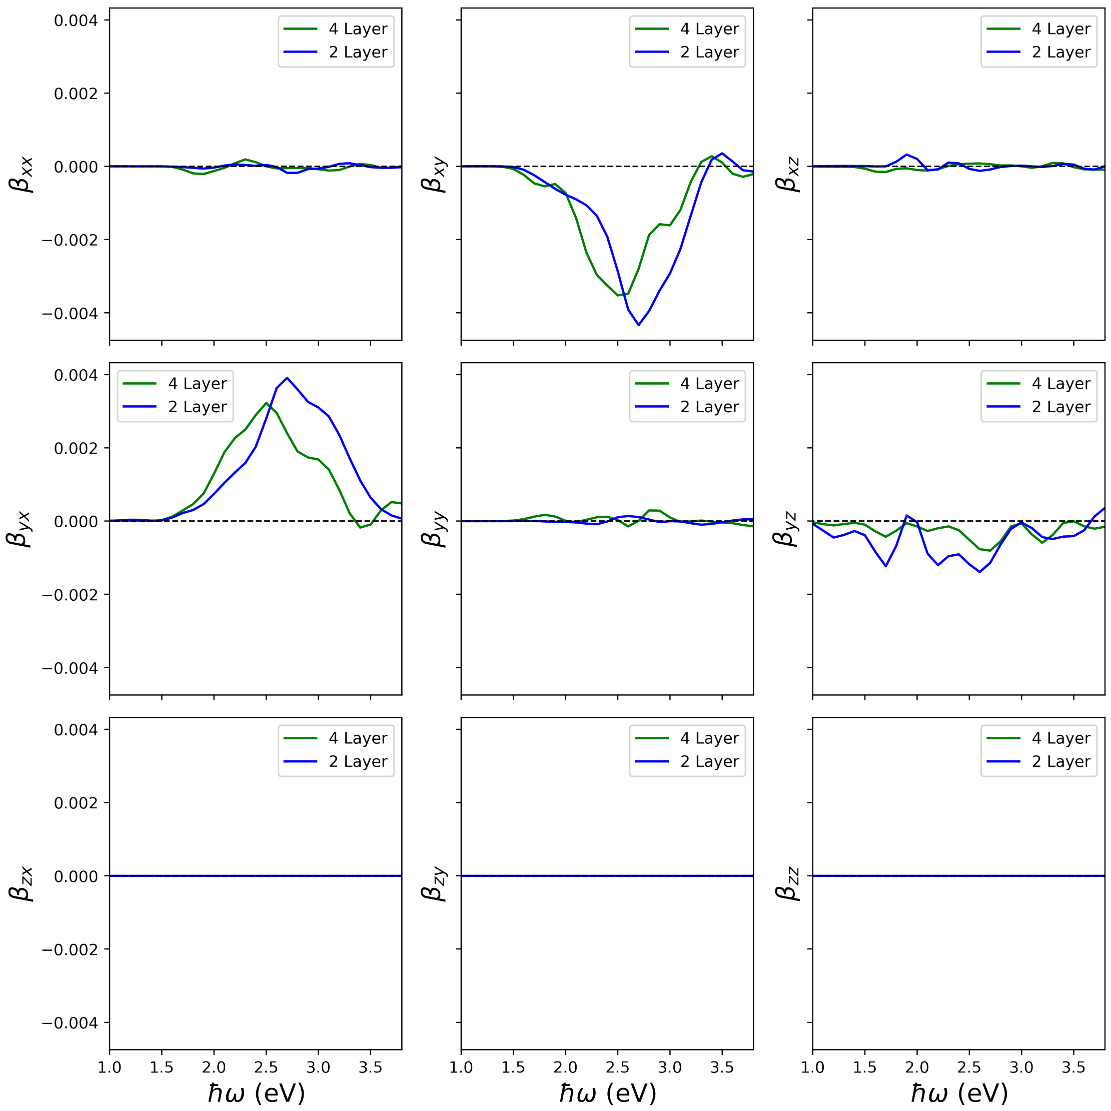


**Figure S 10.** The frequency dependence of individual components of the CPGE tensor ($\beta_{ij}$), $i$ and $j$ are indicated in the y-axis label. 2 Layer represents results from the slab with 2 layers (see Fig. S 8 (a)) and 4 layer is a slab twice as thick as the 2 layer case.

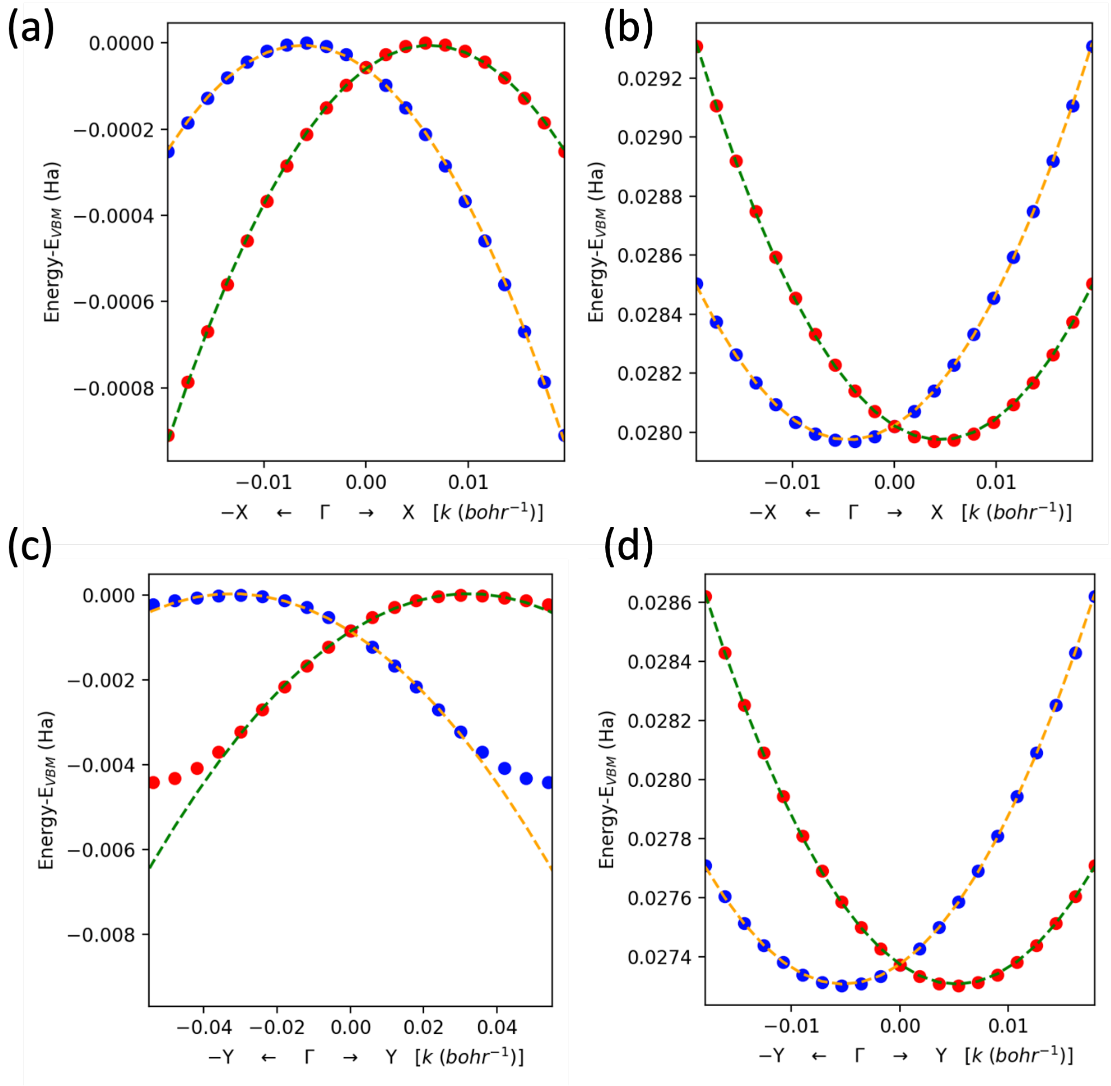


**Figure S 11.** Fitted DFT bands with the dashed lines representing the least squares fit to equation S4 and points representing the DFT results. a) and b) are the in the $k_x$ direction while c) and d) are in the $k_y$ direction. a) and c) are valence bands and b) and d) are conduction bands.

## 2 Hamiltonian modelling of nonlinear photocurrents

We use a 4 band model for halide perovskite comprising two Rashba-split conduction bands and two Rashba split valence bands, similar to Ref.[5]. This model has a Rashba axis along the surface normal direction ($z$). Inversion symmetry breaking induced by the surface potential leads to the Rashba effect ($\alpha$). We first consider the system bulk optical transition dipoles ($\gamma$) as in Ref.[5], and introduce modifications from the surface potential to the optical transition dipoles in Sec. 2.2 using data from DFT calculations.

In the following, we assume that the applied static field is in the $x$-direction, and the current is measured in the $x$-direction.

To this model we add the breaking of time-reversal symmetry, causing the Rashba Hamiltonian to pick up an additional term ($\beta$) and a splitting to be introduced at the point degeneracies of the Rashba model (Fig. S12). In our experimental scenario, a spin imbalance of excited state carriers is established by the Rashba-Edelstein effect under the presence of an external bias field, resulting in broken time-reversal symmetry. The amount of time-reversal symmetry breaking is proportional to the strength of the external bias field. The Hamiltonian is

$$H = \begin{pmatrix} t_c k^2 + E_g + \beta_c k_z & (ik_x + k_y)\alpha_c & -k_z\gamma & -(ik_x + k_y)\gamma \\ (-ik_x + k_y)\alpha_c & t_c k^2 + E_g - \beta_c k_z & (ik_x - k_y)\gamma & k_z\gamma \\ -k_z\gamma & (-ik_x - k_y)\gamma & -t_v k^2 + \beta_v k_z & (ik_x + k_y)\alpha_v \\ -(-ik_x + k_y)\gamma & k_z\gamma & (-ik_x + k_y)\alpha_v & -t_v k^2 - \beta_v k_z \end{pmatrix} \tag{S5}$$

The wavefunctions for bands 1-4 are:

$$U^{(0)} = \begin{pmatrix} \sin\frac{\phi_{ck}}{2} & \cos\frac{\phi_{ck}}{2} & 0 & 0 \\ -e^{i\theta_k}\cos\frac{\phi_{ck}}{2} & e^{i\theta_k}\sin\frac{\phi_{ck}}{2} & 0 & 0 \\ 0 & 0 & \sin\frac{\phi_{vk}}{2} & \cos\frac{\phi_{vk}}{2} \\ 0 & 0 & -e^{i\theta_k}\cos\frac{\phi_{vk}}{2} & e^{i\theta_k}\sin\frac{\phi_{vk}}{2} \end{pmatrix} \tag{S6}$$

where $e^{i\theta_k} = (-ik_x + k_y)/k_{xy}$ and $\cos\phi_{ck} = \frac{\beta_c k_z}{\sqrt{(\beta_c k_z)^2 + (\alpha_c k_{xy})^2}}$. For each band, the diagonal Berry connections $\xi_{nn} = u^{\dagger}_{nk}(i\nabla_k)u_{nk}$ are

$$\xi_{11} = -\frac{1}{k_{xy}}\cos^2\frac{\phi_{ck}}{2}\hat{\theta}_k \tag{S7}$$

$$\xi_{22} = -\frac{1}{k_{xy}}\sin^2\frac{\phi_{ck}}{2}\hat{\theta}_k \tag{S8}$$

$$\xi_{33} = -\frac{1}{k_{xy}}\cos^2\frac{\phi_{vk}}{2}\hat{\theta}_k \tag{S9}$$

$$\xi_{44} = -\frac{1}{k_{xy}}\sin^2\frac{\phi_{vk}}{2}\hat{\theta}_k \tag{S10}$$

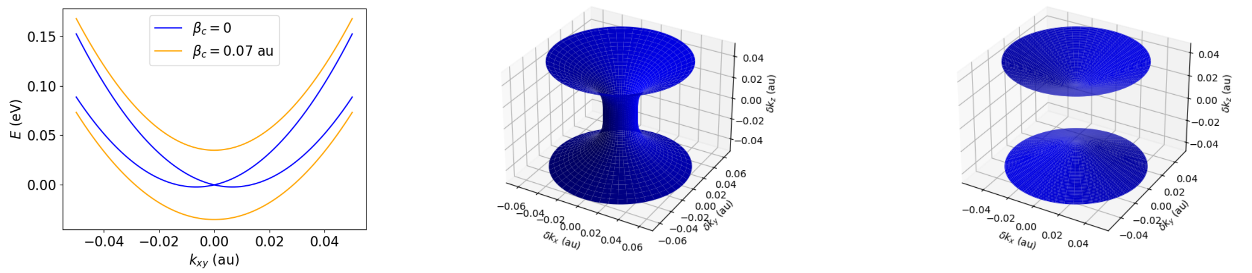


**Figure S 12.** Band structures of model Hamiltonian conduction band (left), showing lifting of Rashba degeneracies upon introduction of time-reversal symmetry breaking terms ($\beta$). Plots of the one-sheet hyperboloid (middle) and two-sheet hyperboloid (right) excitation surfaces, in the vicinity of van Hove singularities. $\delta k = 0$ is the position of the van Hove singularity. The plots are generated with the same band structure parameters used for the model calculations (Section 2.4), at an excitation energy of 0.001 Ha away from the van Hove singularity.

The interband transition dipole matrix elements are $r_{mn} = u^\dagger_{mk}(i\nabla_k)u_{nk} = \frac{1}{\omega_{mn}}u^\dagger_{mk}(i\partial_k H_k)u_{nk}$.

$$r_{mn} = -\frac{i\gamma}{\omega_{mn}} \begin{cases} s(\sin\phi_k \hat{k}_{xy} + \cos\phi_k \hat{k}_z) & s = s' \\ -\cos\phi_k \hat{k}_{xy} + \sin\phi_k \hat{k}_z & s \neq s' \end{cases} \tag{S11}$$

where $\phi_k = (\phi_{ck} + \phi_{vk})/2$ and $\hat{k}_z$ is a unit vector in the positive $k_z$ direction.

The energy dispersion is $E_c = t_c k^2 + s'\sqrt{(\alpha_c k_{xy})^2 + (\beta_c k_z)^2}$ and $E_v = -t_v k^2 + s\sqrt{(\alpha_v k_{xy})^2 + (\beta_v k_z)^2}$. The transition energies $\omega_{mn} = E_c - E_v$ have stationary points (van Hove singularities) at

$$k^*_{xy} = 0 \tag{S12}$$

$$k^*_z = -\frac{s'|\beta_c| - s|\beta_v|}{2(t_c + t_v)} \tag{S13}$$

Near the van Hove singularities, the transition energies can be expanded as

$$\omega_{mn} \approx \omega_0 + \left(t_c + t_v + \frac{s'\alpha_c^2}{2|\beta_c k^*_z|} - \frac{s\alpha_v^2}{2|\beta_v k^*_z|}\right) k^2_{xy} + \mathrm{sgn}(k^*_z)\left(\frac{t_c + t_v}{4|k^*_z|^2}\right)\delta k_z^4 \tag{S14}$$

$$= \omega_0 + A_{xy}k^2_{xy} + A_z \delta k_z^4 \tag{S15}$$

The typical magnitude of $|A_{xy}| \sim t$, and $|A_z| \sim t/k_z^{*2}$. Depending on the signs of the coefficients, these singularities can be either minima ($A_{xy} < 0$, $A_z < 0$), maxima ($A_{xy} > 0$, $A_z > 0$), or saddle points ($A_{xy}A_z < 0$), with all types being possible for all combinations of $s, s'$. For the saddle point singularity $A_{xy} < 0$, $A_z > 0$, the excitation surface forms a one-sheet hyperboloid in the Brillouin zone for $\omega - \omega_0 < 0$ and a two-sheet hyperboloid for $\omega - \omega_0 > 0$ (Fig. S 12). The order is reversed for the other type of saddle point singularity $A_{xy} > 0$, $A_z < 0$ .

## 2.1 Magnetic shift current

In systems with broken time-reversal symmetry, magnetic shift current is possible under circularly polarized light[1]. This results in an effective 3rd order photocurrent which is proportional to the external bias field ($E_0$) controlling the amount of time-reversal symmetry breaking ($\beta$), and proportional to the light intensity $E^2$ controlling the amount of magnetic shift current. The magnetic shift current is

$$\sigma^{abc} = \frac{ie^3}{8\pi^2\hbar^2} \int d^3k \sum_{mn} f_{mn}(r^b_{nm;a} r^c_{mn} + r^c_{nm;a} r^b_{mn})\delta(\omega - \omega_{nm}) \tag{S16}$$

The covariant derivatives of the transition dipoles are defined as

$$r^b_{mn;a} = \frac{dr^b_{mn}}{dk^a} - i(\xi^a_{mm} - \xi^a_{nn})r^b_{mn} \tag{S17}$$

At normal incidence, the relevant tensor element is $a = x$, $b = x$, $c = y$, and the magnetic shift current vanishes because the integrand vanishes when integrated over $k_{xy}$ . This is because of the $C_2$ rotation axis in the z-direction: $r^y$ changes sign on the rotation $k_x \to -k_x, k_y \to -k_y$. Away from normal incidence, the relevant tensor element is $a = x$, $b = x$, $c = z$. In general, this tensor element will not be zero because of the inversion symmetry breaking in the $z$-direction. Therefore, we expect the magnetic shift current to exhibit the same incidence angle dependence of the experiment.

Under a reversal of external bias, we expect the signs of the $\beta_c$ and $\beta_v$ coefficients to change by a negative sign, because of the reversal of the spin populations under the Rashba-Edelstein effect. Then, $\cos\phi_{ck}$ and $\cos\phi_{vk}$ will also change by a negative sign. As we will show in the next section, this will result in a reversal of the current direction, agreeing with the experimental observation.

## 2.2 DFT-fitted transition dipoles

From DFT calculations, we find that the $z$ transition dipoles pick up a strong inversion breaking term from the surface which increases as $k_{xy} \to 0$ (Fig. S 13). Therefore, we add an additional term to the transition dipole matrix elements in the $z$-direction ($\eta$) to describe this effect. This, in combination with van Hove singularities at the same k-point, is responsible for the large magnetic shift currents. The DFT $z$-dipole matrix elements fit well to the form

$$r^z_{mn} = \frac{\eta}{k_{xy}} + O(1) \tag{S18}$$

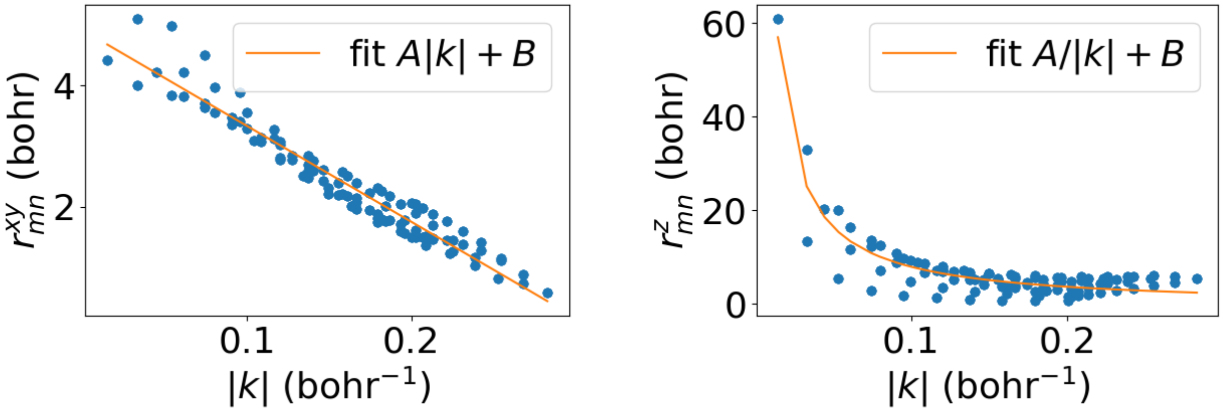


**Figure S 13.** DFT calculated and fitted transition dipole matrix elements in the $xy$ and $z$ directions. Here $r^{xy}$ denotes the magnitude of $r$ in the $xy$ plane. $|k|$ denotes the $k$-vector distance from the $\Gamma$ point in the DFT calculations.

The DFT $xy$-dipole matrix elements have a leading term which is consistent with our bulk model (Eq. S11)

$$r^x_{mn} = \gamma' \cos\phi_k \cos\theta_k + O(k_{xy}) = \gamma' \cos\phi_k \frac{k_x}{\sqrt{k_x^2 + k_y^2}} + O(k_{xy}) \tag{S19}$$

where we have written $\gamma' = i\gamma/\omega_{mn}$. The covariant derivatives are

$$r^x_{mn;x} = \cos\phi_k \gamma' \left( \frac{1}{\sqrt{k_x^2 + k_y^2}} + \frac{k_x^2}{(k_x^2 + k_y^2)^{3/2}} \right) - i\frac{1}{k_{xy}} \cos^2\frac{\phi_{ck}}{2} \frac{k_y}{\sqrt{k_x^2 + k_y^2}} r^x_{mn} \tag{S20}$$

$$\sim \frac{\cos\phi_k \gamma'}{k_{xy}} \tag{S21}$$

where we have discarded all but the divergent part as $k_{xy} \to 0$. From this we see that the term $r^x_{mn;x} r^z_{nm}$ will contribute strongly to the magnetic shift current, and it would change sign under reversal of bias as it is proportional to $\cos\phi_k$. We now consider the magnetic shift current response for the saddle point singularities as they have the largest density of states. For the one-sheet hyperboloid, it is

$$|\sigma^{xxz}| = \frac{e^3}{4\pi^2\hbar^2} |\gamma'||\eta| \int_{k\to k^*} d^3k \frac{1}{k_{xy}^2} \delta(\omega - \omega_{nm}) \tag{S22}$$

$$= \frac{e^3}{2\pi\hbar^2} |\gamma'||\eta| \iint_{k\to k^*} dk_z dk_{xy} \frac{1}{k_{xy}} \left| \frac{d\omega_{mn}}{dk} \right|^{-1}_{k_{xy}=k'_{xy}} \delta(k_{xy} - k'_{xy}) \tag{S23}$$

$$= \frac{e^3}{2\pi\hbar^2} |\gamma'||\eta| \iint_{k\to k^*} dk_z dk_{xy} \frac{\sqrt{A_{xy}}}{\sqrt{(\omega - \omega_0 - A_z\delta k_z^4)}} \frac{\delta(k_{xy} - k'_{xy})}{\sqrt{4A_{xy}(\omega - \omega_0 - A_z\delta k_z^4) + (4A_z\delta k_z^3)^2}} \tag{S24}$$

where $k'_{xy} = \sqrt{(\omega - \omega_0 - A_z \delta k_z^4)/A_{xy}}$. For the two-sheet hyperboloid,

$$|\sigma^{xxz}| = \frac{e^3}{2\pi\hbar^2}|\gamma'||\eta| \iint_{k\to k^*} dk_{xy} dk_z \frac{1}{k_{xy}} \left|\frac{d\omega_{mn}}{dk}\right|^{-1}_{k_z=k'_z} \delta(k_z - k'_z) \tag{S25}$$

$$= \frac{e^3}{2\pi\hbar^2}|\gamma'||\eta| \iint_{k\to k^*} dk_{xy} dk_z \frac{1}{k_{xy}} \frac{\delta(k_z - k'_z)}{\sqrt{(2A_{xy}k_{xy})^2 + 16A_z^2((\omega - \omega_0 - A_{xy}k_{xy}^2)/A_z)^{3/2}}} \tag{S26}$$

where $k'_z = (\omega - \omega_0 - A_{xy}k_{xy}^2)/A_z)^{1/4}$.

Using DFT-derived parameters for the gapped Rashba model (Sec. 2.4), we obtain a strong magnetic shift current (Fig. S 14) which is about two orders of magnitude larger than the 2nd-order injection current. While this simple model predicts magnetic shift current strongly peaked at the energy of the van Hove singularities, there are a few reasons why the current response may not be as strongly peaked in energy. In actual samples, the spin density varies with depth below the surface, which results in the $\beta$ parameters being depth-dependent, smearing out the divergence of the spectrum. Secondly, disorder in the sample may result in the signs of $A_{xy}$ and $A_z$ flipping in different parts of the sample. This results in the order of one-sheet and two-sheet hyperboloid van Hove singularities flipping, giving rise to broadening of the peak. Finally, the simple model presented here only includes the divergent part of the response, while other sub-leading terms should contribute to a broader spectrum. Nevertheless, we expect that the current to peak at frequencies where most of the van Hove singularities lie. This characteristic energy scale of $\sim 100$ meV is the typical energy difference between the band edges and the Rashba model band degeneracy, which is broken by the Rashba-Edelstein effect.

For a fixed external bias value, the direction of the magnetic shift current is fixed by the signs of the $\beta$ parameters (see Eq. S S20 which depends on $\beta_c$ and $\beta_v$ through $\cos\phi_k$). As we see in Fig. S 14, the direction of the magnetic shift current is not expected to change over the frequency range, although its magnitude is greatly diminished away from the van Hove singularities. In comparison, the injection current has a weaker frequency dependence. As a result, depending on the sign of the $\beta$ parameters, it is possible for the total photocurrent to switch direction across the frequency range, as the relative importance of the the magnetic shift current and the injection current components changes. Such changes in the sign of the photocurrent could possibly contribute to the experimentally measured frequency dependence.

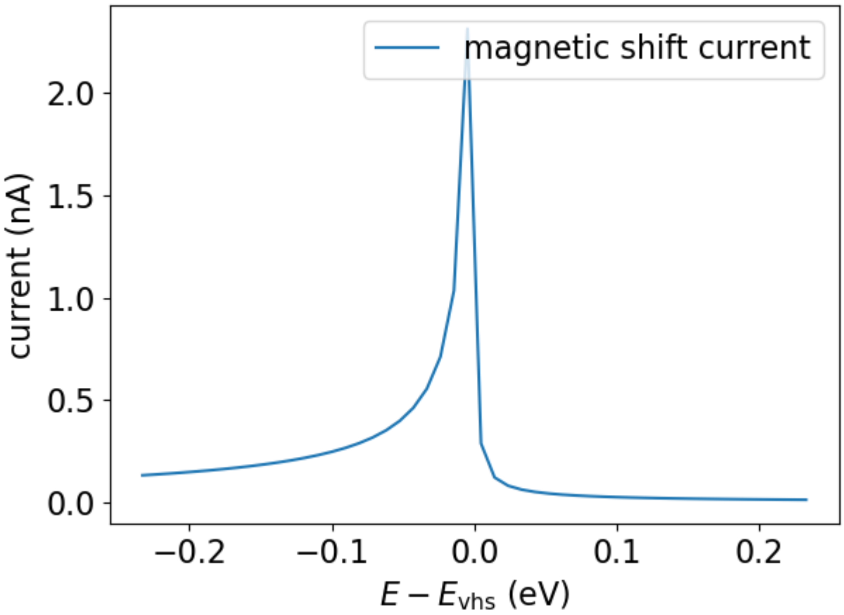


**Figure S 14.** Frequency dependence of magnetic shift current, which has a divergence at the van Hove singularity $E_{\rm vhs}$.

## 2.3 Third-order photocurrents

We consider the third order jerk, injection, and shift currents arising under a static electric field $E_0$ (Ref. [2]).

$$\frac{d}{dt^2}J^a_{jerk} = 6\iota_{abcd}E^bE^cE^d_0 \tag{S27}$$

$$\frac{d}{dt}J^a_{inj} = 6\eta_{abcd}E^bE^cE^d_0 \tag{S28}$$

$$\frac{d}{dt}J^a_{sh} = 6\sigma_{abcd}E^bE^cE^d_0 \tag{S29}$$

For these mechanisms, we set the time-reversal symmetry breaking $\beta = 0$, and consider the response arising solely from the original Rashba model in a static field without any Rashba-Edelstein effect. This group of mechanisms would also scale linearly with the applied static field, and linearly with the intensity of light.

However, the symmetry of the $C_2$ rotation axis in the z-direction results in these response functions vanishing for the experimental geometry. For incidence angles away from normal incidence, the relevant tensor element is $a = x$, $b = x$, $c = z$, $d = x$. The above symmetry dictates that $r^x$ changes sign under the rotation $k_x \to -k_x, k_y \to -k_y$. As a result, all integrals over $k_{xy}$ vanish for these response functions.

Even if this $C_2$ symmetry is broken in the samples, we expect that the magnitude of these third order currents to be small compared to the second order injection current. To show this, we consider the magnitude of the jerk current, which was the largest component of the third order response for the models in Ref.[2]. We consider the jerk current for a model with band dispersion and transition dipoles similar to halide perovskites, but without any symmetries.

The expression for the jerk current response tensor is

$$\iota^{abcd} = \frac{e^4}{6\hbar^3(2\pi)^2}\int d^3k \sum_{mn} f_{mn}\omega_{nm;ad}r^b_{nm}r^c_{mn}\delta(\omega-\omega_{nm}) \tag{S30}$$

A rough estimate for the jerk current is

$$J \sim \tau^2 \frac{e^4}{6\hbar^3(2\pi)^2}(2\text{spin})\frac{d^2\omega}{dk^2}|r|^2 4\pi k^2 \left(\frac{d\omega}{dk}\right)^{-1} E^2 E_0 \tag{S31}$$

where $\frac{d^2\omega}{dk^2}$, $\frac{d\omega}{dk}$, $k$ are the band curvature, velocity, and k-vector at the excitation surface. The current density is $J = 2.0710^{-21}au$. Using a cross section of $0.5\mu m^2$ (Section 2.4), we obtain a photocurrent of 0.0032 pA, which is small compared to the second order injection current. Furthermore, in such a system with no symmetries, the jerk current is not expected to vanish at normal incidence, and would not show the incidence angle dependence of the experiment.

## 2.4 Parameters for numerical estimates

For numerical estimates of the Rashba model photocurrent, we use parameters (in atomic units): $\tau = 119fs = 4917a.u.$. We calculate the band masses in DFT, averaging over $k_x$ and $k_y$ directions to obtain an estimate of the reduced mass: $\frac{d^2\omega}{dk^2} = \frac{1}{m_r} = \frac{1}{m_e} + \frac{1}{m_h} = 7.08$. We use excitation above gap = 0.233 eV = 0.00856 Ha, $k = \sqrt{2m_r\omega} = 0.0492$ , $\frac{d\omega}{dk} = \frac{k}{m_r} = 0.308$, $r = 0.5$ on the excitation surface, $E = 10^3V/m = 1.95 \times 10^{-9}au$ , $E_0 = 10^4V/m = 1.95 \times 10^{-8}au$. To calculate the total current from the current density, we use a cross section of $0.5\mu m^2 = 1.79 \times 10^8 au$. This was obtained by estimating the surface layer thickness using a Debye length on the order of 100 nm, and the width of the spot as 5 $\mu$m.

For the gapped Rashba model, we use $\alpha_c = 0.0234$, $\alpha_v = 0.0362$, $\gamma' = 5.0$, $\eta = 0.857$, all of which are fit to DFT data. For $\alpha_c$ and $\alpha_v$, we use an average of values in the $k_x$ and $k_y$ directions. Besides those parameters, we use $\beta_c = 0.07$, $\beta_v = 0.06$ for the time-reversal degeneracy breaking of the Rashba model. These $\beta$ values correspond to a degeneracy breaking of about 50 meV, consistent with the picture that any modifications to the band structure from the Rashba-Edelstein effect only occur

close to the band edges. We find that fine-tuning of $\beta_c$ relative to $\beta_v$ is not needed to achieve large magnetic shift currents as the mechanism only requires the existence of the van Hove singularities and not any kind of parameter matching between valence and conduction bands; these values were only chosen as examples of the likely magnitude of these parameters.

# References


[1] Haowei Chen, Meng Ye, Nianlong Zou, Bing-Lin Gu, Yong Xu, and Wenhui Duan. Basic formulation and first-principles implementation of nonlinear magneto-optical effects. *Physical Review B*, 105(7):075123, February 2022. Publisher: American Physical Society.

[2] Benjamin M. Fregoso. Bulk photovoltaic effects in the presence of a static electric field. *Physical Review B*, 100(6):064301, August 2019. Publisher: American Physical Society.

[3] Kevin F. Garrity, Joseph W. Bennett, Karin M. Rabe, and David Vanderbilt. Pseudopotentials for high-throughput dft calculations. *Computational Materials Science*, 81:446–452, 2014.

[4] Paolo Giannozzi, Stefano Baroni, Nicola Bonini, Matteo Calandra, Roberto Car, Carlo Cavazzoni, Davide Ceresoli, Guido L Chiarotti, Matteo Cococcioni, Ismaila Dabo, Andrea Dal Corso, Stefano de Gironcoli, Stefano Fabris, Guido Fratesi, Ralph Gebauer, Uwe Gerstmann, Christos Gougoussis, Anton Kokalj, Michele Lazzeri, Layla Martin-Samos, Nicola Marzari, Francesco Mauri, Riccardo Mazzarello, Stefano Paolini, Alfredo Pasquarello, Lorenzo Paulatto, Carlo Sbraccia, Sandro Scandolo, Gabriele Sclauzero, Ari P Seitsonen, Alexander Smogunov, Paolo Umari, and Renata M Wentzcovitch. Quantum espresso: a modular and open-source software project for quantum simulations of materials. *Journal of Physics: Condensed Matter*, 21(39):395502, sep 2009.

[5] Xiaojie Liu, Ashish Chanana, Uyen Huynh, Fei Xue, Paul Haney, Steve Blair, Xiaomei Jiang, and Z. V. Vardeny. Circular photogalvanic spectroscopy of Rashba splitting in 2D hybrid organic–inorganic perovskite multiple quantum wells. *Nature Communications*, 11(1):323, January 2020. Number: 1 Publisher: Nature Publishing Group.

[6] J. E. Sipe and A. I. Shkrebtii. Second-order optical response in semiconductors. *Phys. Rev. B*, 61:5337–5352, Feb 2000.

[7] Ravishankar Sundararaman, Kendra Letchworth-Weaver, Kathleen A. Schwarz, Deniz Gunceler, Yalcin Ozhabes, and T.A. Arias. Jdftx: Software for joint density-functional theory. *SoftwareX*, 6:278–284, 2017.

[8] M.J. van Setten, M. Giantomassi, E. Bousquet, M.J. Verstraete, D.R. Hamann, X. Gonze, and G.-M. Rignanese. The pseudodojo: Training and grading a 85 element optimized norm-conserving pseudopotential table. *Computer Physics Communications*, 226:39–54, 2018.

[9] Junqing Xu, Kejun Li, Uyen N Huynh, Mayada Fadel, Jinsong Huang, Ravishankar Sundararaman, Valy Vardeny, and Yuan Ping. How spin relaxes and dephases in bulk halide perovskites. *Nature Communications*, 15(1):188, 2024.
